# Supplementary material for: Colloidal particle adsorption at water/water interfaces with ultra-low interfacial tension
Source: arXiv:1711.10024 ancillary file (2017-11-29)
Supplement: Supplementary file 1 [file SupplementalMaterial.pdf]

# Supplemental Material:

# Colloidal particle adsorption at water/water interfaces with ultra-low interfacial tension

*Louis Keal[1], Carlos E. Colosqui[2,3], Hans Tromp[4,5], and Cécile Monteux[1]*

[1] ESPCI Paris, PSL Research University, Sciences et Ingénierie de la Matière Molle (SIMM), CNRS UMR 7615, 75231 Paris, France
[2] Department of Mechanical Engineering, Stony Brook University, Stony Brook, NY 11794, USA
[3] Department of Applied Mathematics & Statistics, Stony Brook University, Stony Brook, NY 11794, USA
[4] Van't Hoff Laboratory for Physical and Colloid Chemistry, Utrecht University, 3584CH Utrecht, The Netherlands
[5] NIZO Food Research, Kernhemseweg 2, 6718 ZB Ede, The Netherlands

## 1. DAMPING COEFFICIENTS

The damping coefficient determines the dissipative forces acting on the adsorbed particles and is an important component of the proposed analytical model (Eqs. 1-4 in the main text) to quantitatively describe the (initial) capillary driven and (late) thermally activated regimes observed in our experiments. In this section we report damping coefficients obtained from the observed particle trajectories and compare them against predictions from conventional models for dynamic contact lines.

Following ideas proposed in prior work by Colosqui *et al.* [1, 2], we consider that the center of mass position $z(t)$ of a colloidal particle with nanoscale surface "defects" can be modeled by a Langevin equation

$$m_p \frac{d^2 z}{dt^2} = -f_d \frac{dz}{dt} - \frac{\partial \mathcal{F}}{\partial z} + \sqrt{2 k_B T f_d}\, \eta(t), \qquad \text{(SM1)}$$

where $m_p$ is the particle mass, $f_d(z)$ is the local damping coefficient accounting for energy dissipation, and $\mathcal{F}$ (see Eq. 1 in the main text) is the system free energy determined by the work of conservative forces. The last term in Eq. SM1, where $\eta$ is Gaussian noise with zero mean and unit variance, considers the effects of thermal fluctuations in a system with constant thermal energy $k_B T$. When a particle is sufficiently far from the equilibrium position $z_E$ there are no local minima in the free energy profile $\mathcal{F}(z)$ (i.e., no metastable positions) and one can neglect the effects of nanoscale surface defects on the average particle trajectory. For particles adsorbed from below the interface this condition (see Eq. 5 in the main text) is given by

$$z \leq z_E - \alpha\pi \frac{\Delta\mathcal{F}}{\gamma A_d}, \qquad \text{(SM 2)}$$

where $\Delta\mathcal{F}$ is the characteristic energy barrier induced by the surface defects, $A_d$ is the projected defect area (see Table 2 in the main text), and a factor $\alpha = 0.5$ approximately predicts the crossover position to a regime dominated by thermally activated transitions between metastable states.

For particle position satisfying Eq. SM2, we find that $\partial\mathcal{F}/\partial z \simeq 2\gamma\pi R(\cos\theta - \cos\theta_E)$; here, $\gamma$ is the surface tension of the water/water (W/W) interface, $R$ is the particle radius, and $\theta$ and $\theta_E$ are the non-equilibrium and equilibrium contact angles, respectively. Further ignoring inertial effects, the damping coefficient in Eq. SM1 satisfies the relation

$$f_d = -2\pi R\gamma \frac{(\cos\theta - \cos\theta_E)}{\langle dz/dt \rangle}, \qquad \text{(SM3)}$$

where the brackets $\langle\ \rangle$ indicate ensemble average. Using Eq. SM3 and assuming a flat interface, for which $z = R\cos\theta$, one can readily obtain local damping coefficients $f_d(z)$ from the observed averaged particle trajectories $\langle z(t)\rangle$. As reported in Fig. SM1, local damping coefficients estimated via Eq. SM3 are nearly position independent after a short initial dynamics for which inertial effects cannot be neglected and before the gradual crossover to the thermally activated regime predicted by Eq. SM2 for $\alpha < 0.5$ (see horizontal dashed lines in Fig. SM1). Damping coefficients for the studied particle radii $R = 0.5$-$6$ $\mu$m are closely described by the relation $f_d = 6\pi\mu_e R$ (cf. Fig. SM1), where the effective viscosity $\mu_e \simeq 6.12\,\mu$ is about six times larger than the shear viscosity $\mu = 0.515$ Pa s of the gelatin-rich phase. It is worth noticing that as the particle motion becomes dominated by thermally activated transitions between metastable states, Eq. SM3 ceases to be valid and the experimentally estimated damping coefficients seem to diverge (cf. Fig.1).

Experimental results for $f_d$ obtained via Eq. SM3 can be directly compared against analytical models such as the Voinov-Cox (VC) model [3, 4], which considers strong hydrodynamic damping near the contact line, and the Molecular Kinetic Theory (MKT) by Blake and coworkers [5, 6], which considers that energy is dissipated during the thermally activated adsorption and desorption of fluid molecules when the contact line moves over a solid surface. When using both VC and MKT models we will only consider contributions from the gelatin-rich phase

because the viscosity $\mu$ of this phase is over 12 times larger than that of the dextran-rich phase.

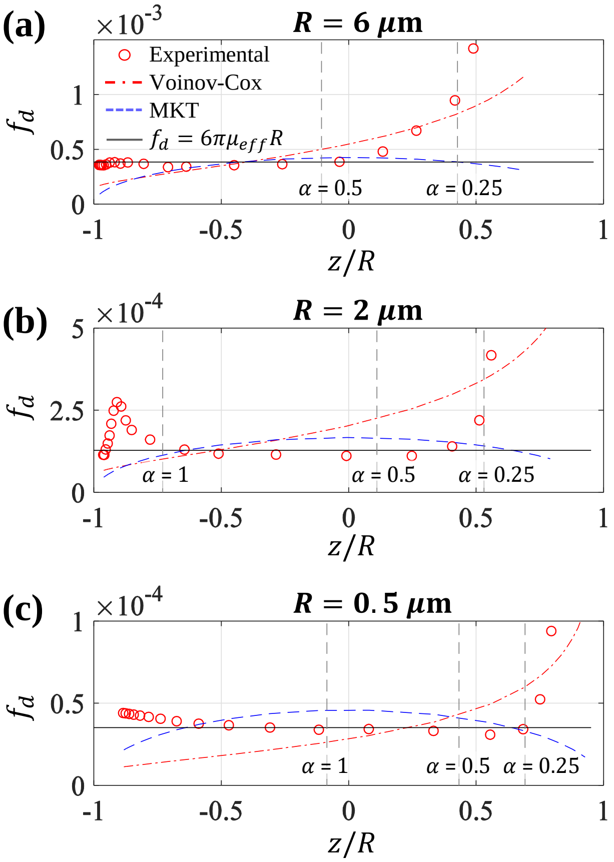


Figure 1: Damping coefficient $f_d(z)$. (a) $R = 6\ \mu$m. (b) $R = 2\ \mu$m. (c) $R = 0.5\ \mu$m.. Vertical dash lines indicate crossover positions predicted from Eq. SM2 for $\alpha$ =0.25-1.0.

According to the V-C model the non-equilibrium contact angle is given by the relation

$$\theta^3 = \theta_E^3 + 9\frac{\mu}{\gamma}\frac{dz}{dt}\ln\left(\frac{L}{\epsilon}\right), \qquad \text{(SM4)}$$

where the macroscopic length $L$ is estimated as the capillary length of the studied system, and $\epsilon$ is the microscopic cutoff length, which is an adjustable model parameter. The damping coefficients predicted by the V-C model are obtained by using Eq. SM4 in Eq. SM3. As reported in Fig .1 the variation of damping coefficients with position predicted by the V-C model is in poor agreement with experimental observations. Moreover, the best least-mean-square fits to the experimental data by V-C predictions (cf. Fig. SM1) is produced by using unphysically small cutoff lengths $\epsilon$ = 4.1-72.6 pm.

The so-called MKT by Blake & Hynes predicts a local damping coefficient

$$f_d = \chi\mu 2\pi R\sqrt{1-\left(\frac{z}{R}\right)^2} \qquad \text{(SM5)}$$

determined by the factor $\chi = (\nu/\lambda_M^3)\exp(-\gamma\lambda_M^2(1+\cos\theta_E)/k_BT)$; here, $\nu$ is the molecular volume of the adsorbed fluid, and $\lambda_M$ is the characteristic size of adsorption sites on the solid surface. The best least-mean-square fits to the experimentally estimated damping coefficients are obtained for factors $\chi \simeq$20-23. These values correspond to adsorption site sizes $\lambda_M = 0.17 \pm 0.03$ nm, when $\nu = 29.8$ Å$^3$ is given by the molecular volume of water. Similar factor magnitude $\chi \sim 20$ can be obtained for much larger adsorption sites when employing larger values of the molecular volumes $\nu$. In any case, damping coefficients predicted by MKT (Eq. SM5) show a significant decrease far from the interface at $z = 0$ (cf. Fig. SM1,) that is not consistent with the local damping coefficient obtained from experimental observations via Eq. SM3. Based on the analysis of local damping coefficients presented in this section we adopted a position-independent damping coefficient to model the dissipative forces on the adsorbed particles. As discussed in the main text, a position-independent damping coefficient can be attributed to topological hindrance due to interactions of adsorbed polymer chains on the particle surface with the surrounding matrix of the semi-dilute gelatin and dextran solutions, which have a similar topological structure.

## 2. GELATIN ADSORPTION

In this section, we present measurements performed to determine whether dextran and/or gelatin are adsorbed on the surface of the studied latex particles.

### 2.1. Total Organic Carbon measurements

The Total Organic Carbon (TOC) content of the studied solutions is measured with a Shimadzu TOC-V CSH machine. Latex particles are added to polymer solutions of known concentration. The suspension is then centrifuged to obtain the supernatant. The total amount of polymer present in the supernatant is then measured, by injecting small quantities of the solution into a high temperature micro-oven, and measuring the resulting heat generated through oxidation of the carbon atoms. By comparing the obtained signal to a calibration curve obtained for a series of polymer solutions of known concentration, one can then deduce the amount of polymer in the supernatant and subsequently the amount of polymer adsorbed on the particles.

In our TOC measurements, particles are added to a polymer solution, with concentrations chosen such that in the case of no polymer adsorption (i.e. maximum carbon content) the signal received by the TOC measurement is

high enough to allow good resolution, but not too high to saturate the detector. The particle concentration is chosen in such manner that under reasonable assumptions of surface coverage upon polymer adsorption, the polymer concentration in the supernatant will vary significantly.

Table SM1 summarizes TOC results from our measurements. The studied dextran solutions showed a weak difference in carbon content before and after addition of particles, which implies that dextran may adsorb very weakly on the particles. On the other hand, fish gelatin showed no carbon remaining in the supernatant, implying that fish gelatin strongly adsorbs to sulfate latex particles.

Table SM1: Total Organic Carbon measurements.

| **Probed phase** | **Latex Particles** | **Polymer initial** | **Polymer Supernatant** |
|---|---|---|---|
| Dextran | 0.001 wt% | 0.005 wt% | 0.0043 wt% |
| Dextran | 0.001 wt% | 0.0125 wt% | 0.0124 wt% |
| Gelatin | 0.0002% wt | 0.05 wt% | 0.000 wt% |

### 2.2. Zeta potential measurements

To further probe the adsorption of polymers on the latex particles, we measured their zeta potential in the presence of gelatin, dextran, and both polymers mixed. Our measurements are performed using a Malvern Zetasizer. The particles are initially dispersed in Milli-Q water before being added to a highly dilute polymer stock, and the samples are shaken vigorously. After this, 30 minutes is allowed for polymer diffusion before zeta potential measurements are taken.

Table SM2: Zeta potential measurements (mean$\pm$std)

| **Sample** | **z-potential** |
|---|---|
| 0.01% Fish Gelatin | 3.8$\pm$3 mV |
| 0.01% Latex | -33$\pm$6 mV |
| 0.01% Latex +0.25% dextran | -34$\pm$5.5 mV |
| 0.01% Latex +0.0165% gelatin | 0.2$\pm$2.2 mV |
| 0.01% Latex +0.165% gelatin | 9$\pm$3.5 mV |
| 0.01% Latex +0.25% gelatin+0.0165% dextran | -1.5$\pm$3.5 mV |
| 0.01% Latex +0.25% gelatin+0.165% dextran | 7$\pm$3.5 mV |
| 0.01% Latex +85mM NaCl | -33$\pm$6 mV |
| 0.01% Latex +85mM NaCl+ 0.0165% gelatin | -0.1$\pm$4 mV |

Table SM2 presents values of the zeta potential for various concentrations of latex, gelatin, and dextran in % w/w. Results in Table SM2 show that fish gelatin has a weak positively charge, and the sulfate latex particles are negatively charged. Upon addition of fish gelatin in the latex particle suspension, the measured zeta potential of the particles becomes slightly positive. These observations indicate that gelatin adsorbs on the surface of the latex particles, which leads to the observed charge reversal of the particle’s zeta potential. When immersed in dextran solutions, the zeta potential of the particles does not change significantly. Both our zeta potential and TOC measurements thus indicate that dextran does not adsorb significantly on the latex particles. When fish gelatin is added to the latex/dextran suspension, the particles’ zeta potential goes from -34 mV to -1.5 or +7 mV for 0,0165 and 0,165% w/w of gelatin concentrations, respectively. The zeta potential measured for particle/gelatin suspensions is the same within error bars in the presence or absence of dextran. This seems to indicate that gelatin adsorption on the latex particles is not affected by the presence of dextran in solution.

When adding salt to the fish gelatin/latex solution, the measured zeta potential decreases slightly from 9mV to 0mV but remains much higher than the one measured for the latex particles in water. Since addition of salt results in the screening of surface charges, we can infer that electrostatic interactions influence to some extent the adsorption of gelatin on the charged latex surfaces. However, based on zeta potential measurements presented in Table SM2, salt in large concentration of 85 mM does not prevent the adsorption of gelatin on the latex surfaces. These observations indicate that hydrophobic interactions are likely to dominate the adsorption of gelatin on the particles as reported in previous work [7].

## REFERENCES


1. C. E. Colosqui, J. F. Morris, and J. Koplik, Phys. Rev. Lett. 111, 028302 (2013).
2. A. M. Rahmani, A. Wang, V. N. Manoharan, and C. E. Colosqui, Soft Matter 12, 6365 (2016).
3. O. Voinov, Fluid Dynamics 11, 714 (1976).
4. R. Cox, J. Fluid Mech. 168, 169 (1986).
5. T.D. Blake and J. Haynes, J. Colloid Interface Sci. 30, 421 (1969).
6. T.D. Blake, J. Colloid Interface Sci., 299, 1, (2006).
7. S. F. Turner, S. M. Clarke, A. R. Rennie, P. N. Thirtle, Z. X. Li, R. K. Thomas, S. Langridge, and J. Penfold, Langmuir 21, 10082 (2005).
